# Supplementary material for: Is it an i or an l: Test-time Adaptation of Text Line Recognition Models
Source: arXiv:2308.15037 source file (2023-08-29)
Supplement: Supplementary file 1 [file supplementary.tex]

% %File: anonymous-submission-latex-2024.tex
% \documentclass[letterpaper]{article} % DO NOT CHANGE THIS
% \usepackage{aaai24}  % DO NOT CHANGE THIS
% \usepackage{times}  % DO NOT CHANGE THIS
% \usepackage{helvet}  % DO NOT CHANGE THIS
% \usepackage{courier}  % DO NOT CHANGE THIS
% \usepackage[hyphens]{url}  % DO NOT CHANGE THIS
% \usepackage{graphicx} % DO NOT CHANGE THIS
% \urlstyle{rm} % DO NOT CHANGE THIS
% \def\UrlFont{\rm}  % DO NOT CHANGE THIS
% \usepackage{natbib}  % DO NOT CHANGE THIS AND DO NOT ADD ANY OPTIONS TO IT
% \usepackage{caption} % DO NOT CHANGE THIS AND DO NOT ADD ANY OPTIONS TO IT
% \frenchspacing  % DO NOT CHANGE THIS
% \setlength{\pdfpagewidth}{8.5in} % DO NOT CHANGE THIS
% \setlength{\pdfpageheight}{11in} % DO NOT CHANGE THIS
% %
% % These are recommended to typeset algorithms but not required. See the subsubsection on algorithms. Remove them if you don't have algorithms in your paper.
% \usepackage{epsfig}
% \usepackage{amsmath}
% \usepackage{amssymb}
% \usepackage{multirow}
% \usepackage{comment}
% \usepackage{algorithm}
% \usepackage{algpseudocode}
% \usepackage{nicefrac}
% % \usepackage{color}
% % \usepackage{xcolor}
% \usepackage[table,xcdraw]{xcolor}
% \usepackage{booktabs}
% \usepackage{subcaption}
% \usepackage{pifont}
% \captionsetup[table]{skip=10pt}
% \DeclareMathOperator*{\argmax}{arg\,max}
% \DeclareMathOperator*{\argmin}{arg\,min}
% \newcommand{\SP}[1]{{\color{blue}#1}}
% \usepackage{pifont}
% \newcommand{\cmark}{\ding{51}}%
% \newcommand{\xmark}{\ding{55}}%
% \usepackage[T1]{fontenc}
% % \usepackage{LobsterTwo}
% \newcommand{\xxcomment}[4]{\textcolor{#1}{[$^{\textsc{#2}}_{\textsc{#3}}$ #4]}}
% \newcommand{\gm}[1]{\xxcomment{cyan}{G}{M}{#1}}
% % \renewcommand{\baselinestretch}{0.955}



% % Include other packages here, before hyperref.

% % If you comment hyperref and then uncomment it, you should delete
% % egpaper.aux before re-running latex.  (Or just hit 'q' on the first latex
% % run, let it finish, and you should be clear).
% % \usepackage[breaklinks=true,bookmarks=false]{hyperref}

% %
% % These are are recommended to typeset listings but not required. See the subsubsection on listing. Remove this block if you don't have listings in your paper.
% \usepackage{newfloat}
% \usepackage{listings}
% \DeclareCaptionStyle{ruled}{labelfont=normalfont,labelsep=colon,strut=off} % DO NOT CHANGE THIS
% \lstset{%
% 	basicstyle={\footnotesize\ttfamily},% footnotesize acceptable for monospace
% 	numbers=left,numberstyle=\footnotesize,xleftmargin=2em,% show line numbers, remove this entire line if you don't want the numbers.
% 	aboveskip=0pt,belowskip=0pt,%
% 	showstringspaces=false,tabsize=2,breaklines=true}
% \floatstyle{ruled}
% \newfloat{listing}{tb}{lst}{}
% \floatname{listing}{Listing}
% %
% % Keep the \pdfinfo as shown here. There's no need
% % for you to add the /Title and /Author tags.
% \pdfinfo{
% /TemplateVersion (2024.1)
% }

% % DISALLOWED PACKAGES
% % \usepackage{authblk} -- This package is specifically forbidden
% % \usepackage{balance} -- This package is specifically forbidden
% % \usepackage{color (if used in text)
% % \usepackage{CJK} -- This package is specifically forbidden
% % \usepackage{float} -- This package is specifically forbidden
% % \usepackage{flushend} -- This package is specifically forbidden
% % \usepackage{fontenc} -- This package is specifically forbidden
% % \usepackage{fullpage} -- This package is specifically forbidden
% % \usepackage{geometry} -- This package is specifically forbidden
% % \usepackage{grffile} -- This package is specifically forbidden
% % \usepackage{hyperref} -- This package is specifically forbidden
% % \usepackage{navigator} -- This package is specifically forbidden
% % (or any other package that embeds links such as navigator or hyperref)
% % \indentfirst} -- This package is specifically forbidden
% % \layout} -- This package is specifically forbidden
% % \multicol} -- This package is specifically forbidden
% % \nameref} -- This package is specifically forbidden
% % \usepackage{savetrees} -- This package is specifically forbidden
% % \usepackage{setspace} -- This package is specifically forbidden
% % \usepackage{stfloats} -- This package is specifically forbidden
% % \usepackage{tabu} -- This package is specifically forbidden
% % \usepackage{titlesec} -- This package is specifically forbidden
% % \usepackage{tocbibind} -- This package is specifically forbidden
% % \usepackage{ulem} -- This package is specifically forbidden
% % \usepackage{wrapfig} -- This package is specifically forbidden
% % DISALLOWED COMMANDS
% % \nocopyright -- Your paper will not be published if you use this command
% % \addtolength -- This command may not be used
% % \balance -- This command may not be used
% % \baselinestretch -- Your paper will not be published if you use this command
% % \clearpage -- No page breaks of any kind may be used for the final version of your paper
% % \columnsep -- This command may not be used
% % \newpage -- No page breaks of any kind may be used for the final version of your paper
% % \pagebreak -- No page breaks of any kind may be used for the final version of your paperr
% % \pagestyle -- This command may not be used
% % \tiny -- This is not an acceptable font size.
% % \vspace{- -- No negative value may be used in proximity of a caption, figure, table, section, subsection, subsubsection, or reference
% % \vskip{- -- No negative value may be used to alter spacing above or below a caption, figure, table, section, subsection, subsubsection, or reference

% \setcounter{secnumdepth}{0} %May be changed to 1 or 2 if section numbers are desired.

% % The file aaai24.sty is the style file for AAAI Press
% % proceedings, working notes, and technical reports.
% %

% % Title

% % Your title must be in mixed case, not sentence case.
% % That means all verbs (including short verbs like be, is, using,and go),
% % nouns, adverbs, adjectives should be capitalized, including both words in hyphenated terms, while
% % articles, conjunctions, and prepositions are lower case unless they
% % directly follow a colon or long dash
% \title{Supplementary Material for \\Is it an i or an l: Test-time Adaptation of Text Line Recognition Models}
% \author{
%     %Authors
%     % All authors must be in the same font size and format.
%     % Written by AAAI Press Staff\textsuperscript{\rm 1}\thanks{With help from the AAAI Publications Committee.}\\
%     % AAAI Style Contributions by Pater Patel Schneider,
%     % Sunil Issar,\\
%     % J. Scott Penberthy,
%     % George Ferguson,
%     % Hans Guesgen,
%     % Francisco Cruz\equalcontrib,
%     % Marc Pujol-Gonzalez\equalcontrib
    
%     Debapriya Tula, Sujoy Paul, Gagan Madan, Peter Garst, Reeve Ingle, Gaurav Aggarwal
% }
% \affiliations{
%     %Afiliations
%     Google Research
%     % \textsuperscript{\rm 1}Association for the Advancement of Artificial Intelligence\\
%     % % If you have multiple authors and multiple affiliations
%     % % use superscripts in text and roman font to identify them.
%     % % For example,

%     % % Sunil Issar\textsuperscript{\rm 2},
%     % % J. Scott Penberthy\textsuperscript{\rm 3},
%     % % George Ferguson\textsuperscript{\rm 4},
%     % % Hans Guesgen\textsuperscript{\rm 5}
%     % % Note that the comma should be placed after the superscript

%     % 1900 Embarcadero Road, Suite 101\\
%     % Palo Alto, California 94303-3310 USA\\
%     % % email address must be in roman text type, not monospace or sans serif
%     % proceedings-questions@aaai.org
% %
% % See more examples next
% }

% %Example, Single Author, ->> remove \iffalse,\fi and place them surrounding AAAI title to use it
% \iffalse
% \title{My Publication Title --- Single Author}
% \author {
%     Author Name
% }
% \affiliations{
%     Affiliation\\
%     Affiliation Line 2\\
%     name@example.com
% }
% \fi

% \iffalse
% %Example, Multiple Authors, ->> remove \iffalse,\fi and place them surrounding AAAI title to use it
% \title{My Publication Title --- Multiple Authors}
% \author {
%     % Authors
%     First Author Name\textsuperscript{\rm 1},
%     Second Author Name\textsuperscript{\rm 2},
%     Third Author Name\textsuperscript{\rm 1}
% }
% \affiliations {
%     % Affiliations
%     \textsuperscript{\rm 1}Affiliation 1\\
%     \textsuperscript{\rm 2}Affiliation 2\\
%     firstAuthor@affiliation1.com, secondAuthor@affilation2.com, thirdAuthor@affiliation1.com
% }
% \fi


% % REMOVE THIS: bibentry
% % This is only needed to show inline citations in the guidelines document. You should not need it and can safely delete it.
% \usepackage{bibentry}
% % END REMOVE bibentry

% \begin{document}

% \maketitle

% %-------------------------------------------------------------------------

% % \begin{figure}
% %     \centering
% %     \includegraphics[scale=0.4]{./figures/kohtd.png}
% %     \caption{\textbf{Exemplar from the KOHTD dataset. We use the word level dataset for our evaluations.}}
% %     \label{fig:kohtd_fig}
% % \end{figure}


% % \section{Experiments on KOHTD, a non-Latin dataset.}
% % \textbf{KOHTD} (Kazakh offline Handwritten Text dataset) consists of a large collection of exam papers filled by students in the Kazakh Language (99\%) and Russian Language (1\%). It contains a total of 1891 images, containing word level annotations for each page. A sample image from the dataset is shown in Figure~\ref{fig:kohtd_fig}.

% % In table \ref{table:seg_iter_kohtd}, we show the performance of our method against three baselines and the source model. We can see that our proposed method is able to achieve an average of 6.6 \% improvement in CER across all corrupted versions, including the original one. Detailed analysis for all datasets across all corruptions can be found in subsequent sections.

% \begin{figure*}[h]
%     \centering
%     \includegraphics[scale=0.5]{./figures/qualitative_examples.pdf}
%     \caption{Exemplars showing the predictions over self-training iterations on two images each from the three datasets.}
%     \label{fig:qualitative}
% \end{figure*}

% \section{Exemplars of predictions over progressive self-training iterations}
% Figure \ref{fig:qualitative} shows the predictions after every iteration of the proposed self-training approach. As we can see, the predictions improve over iterations. For example, for the second one from top, the model quickly figures out that the style of `l' looks different from that of `d', and hence it corrects that in the later iterations. Similarly for the third example from the top, the multiple `s' in ``session" get correctly recognized over iterations. We see similar improvements in the other examples as well.

% % \input{./tables/comp_baselines_kohtd}


% \input{./tables_for_supp/icdar/selftrain_complete}
% \input{./tables_for_supp/gnhk/selftrain_complete}
% \input{./tables_for_supp/iam/selftrain_complete}
% \input{./tables_for_supp/cvl/selftrain_complete}
% \input{./tables_for_supp/kohtd/selftrain_complete}


% \section{Category-wise ablation of self-training the optical model}
% In Tables \ref{table:icdar_table}, \ref{table:gnhk_table}, \ref{table:iam_table}, \ref{table:cvl_table} and \ref{table:kohtd_table}, we show ablation results for various choices of our self-training approach. For ICDAR2015-HTR, we observe that our method performs better than the other options for most corruptions. Our augmentation based reweighting strategy with progressive update of labels shows CER improvements of as much as $\textbf{5.6\%}$ (for impulse noise corruption). %The elastic transformation contracts or stretches portions of a line image \cite{hendrycks2019benchmarking}, which leads to large degradation in image quality at the character level. Thus, errors in pseudo-labels generated, can propagate during the self-train process to further degrade the quality of predictions.

% For the GNHK dataset, we observe similar trends as ICDAR2015-HTR. We observe an improvement in CER of as much as $\textbf{4.7\%}$ for the glass blur corruption. On an average, our proposed augmentation based TTA with reweighting performs the best and shows an improvement of $1.3\%$ over the baseline for all corruptions, including the original dataset.

% In case of IAM, we observe that our method performs much better than the other options on average. Our method perform the best for majority of the corruptions, and shows an improvement of as much as $\textbf{7.1}\%$ (for the glass blur corruption). For a few of the corruptions adapting the model using predictions over all lines of an image as pseudo labels helps better. We speculate this happens because IAM being a much easier dataset, the predictions generated from the source model itself are of good quality, and hence serve as good self-labels. Thus, updating the model with the self-labels for all lines, over all iterations performs a bit better.

% For the CVL dataset, we observe improvements in most cases, with a maximum improvement of $\textbf{5.5}$\%, except a few corruptions like defocus\_blur, elastic, gaussian\_blur and zoom\_blur. This can be attributed to the correctness of the self-labels due to the hard inherent distortions these corruptions introduce. 

% In case of the dataset, KOHTD, we observe a consistent improvement across all corruptions. We observe that our progressive update of self-labels with reweighting shows CER improvements of at least $0.3\%$ and as much as $\textbf{8.8}\%$. KOHTD, being a low resource language dataset, we believe that the divergence controlled adaptation we introduce helps identify and learn from the writer's idiosyncrasies very effectively.




% % \section{Results mentioned for ICDAR only in the main paper}
% % Table 2, 3, 4 and Figures 6 and 7 for each GNHK and IAM as well. 

% \section{Understanding the correlation between our confidence metric and correctness.}
% In our algorithm, we use a confidence metric to both rank and weight losses for lines --  which forms the core of our progressive self-training approach. Our confidence metric (which we call the Normalized Edit Distance (NED) in the tables and figures) determines whether the optical model is smooth in the neighborhood of the input image. A baseline confidence metric is the CTC loss itself w.r.t. the top-1 prediction, with which we compare in Tables \ref{table:icdar_table}, \ref{table:gnhk_table}, \ref{table:iam_table}, \ref{table:cvl_table} and \ref{table:kohtd_table}. In order to better understand the usefulness of the proposed confidence metric, we find the correlation of the confidence metric and the CER of the self-labels with the ground-truth. We perform the analysis for both our metric and the CTC loss based weights (normalized over all lines in an image). The plots over the five datasets are shown in Figures \ref{fig:icdar_main_plot}, \ref{fig:gnhk_main_plot}, \ref{fig:iam_main_plot}, \ref{fig:cvl_main_plot} and \ref{fig:kohtd_main_plot}. As we can see from the plots on the right of the figures which represent the confidence scores derived using our augmentation based NED metric, as the CER for a line increases, the confidence of the model over the line also decreases. We see a much higher correlation between the CER and the proposed metric than the confidence based on the CTC loss.


% %todo
% \section{Ablation studies with varying number of iterations}
% We evaluate our method for different number of iterations $K$ of our self-training algorithm. Recall, we progressively add $\frac{m}{K}$ lines to our set of confident lines, where $m$ is the total number of lines in an image. We run our algorithm for $ K \in \{1, 2, 4, 6, 8, 10, 12\}$. The results are shown for all corruptions in tables \ref{table:topx_icdar}, \ref{table:topx_gnhk}, and \ref{table:topx_iam}. As discussed in the paper, when we have very few update iterations, we do not allow the self-training algorithm to improve, and on the other hand, too many iterations may lead to divergence, as the algorithm does not use any ground-truth labels, but learns from self-labels only. We find that for all the datasets, number of iterations $K=4$, i.e., incrementally taking $25\%$ of the lines in each iteration results in the best performance. We can observe that choosing $K=4$ helps us strike the right balance between performance and total number of iterations.

% %todo
% \section{The Impact of LM on TTA}
% In the paper we show this analysis on GNHK, where we find that the performance significantly degrades if we do not use the LM in the self-training loop. This is because the LM acts as a cushion and prevents the model from diverging, which can otherwise happen because of the incorrect self-labels from just the optical model. Here, we show the analysis on two other datasets. When we do not use LM in the self-training algorithm, we observe a drop in performance from $23.9$ to $44.4$ on ICDAR2015-HTR, from $24.7$ to $31.4$ on GNHK, and from $13.6$ to $21$ on IAM. We also show a similar plot as in the paper in Figure \ref{fig:lm_impact} for ICDAR2015-HTR and IAM. The plot shows how the performance improvement offered by the LM on the source model inference can have an impact on the TTA performance. 

% \begin{figure*}
%     \centering
%     \includegraphics[scale=0.25]{./plots_for_supp/icdar/main_plot.png}
%     \caption{\small \textbf{Correlation between correctness and confidence metric used on ICDAR2015-HTR} Plot of ground-truth CER vs the confidence obtained based on the CTC loss (left), and the confidence obtained using our augmentation based confidence metric (right). Our confidence metric assigns higher values to the lines with lower CER. Whereas, for the same CTC loss based confidence, we observe a wide range of CER, indicating a low correlation with correctness.}
%     \label{fig:icdar_main_plot}
% \end{figure*}
% \begin{figure*}
%     \centering
%     \includegraphics[scale=0.25]{./plots_for_supp/gnhk/main_plot.png}
%     \caption{\small \textbf{Correlation between correctness and confidence metric used on GNHK} Plot of ground-truth CER vs the confidence obtained based on the CTC loss (left), and the confidence obtained using our augmentation based confidence metric (right). Our confidence metric assigns higher values to the lines with lower CER. Whereas, for the same CTC loss based confidence, high weights are assigned to the lines irrespective of their CERs, indicating a low correlation with correctness. There is even a positve correlation between the confidence using CTC loss and the CER, which should have been otherwise negative, as more confidence should be assigned to lines with lower CER, i.e., ones which are supposedly less wrong.}
%     \label{fig:gnhk_main_plot}
% \end{figure*}
% \begin{figure*}
%     \centering
%     \includegraphics[scale=0.25]{./plots_for_supp/iam/main_plot.png}
%     \caption{\small \textbf{Correlation between correctness and confidence metric used on IAM} Plot of ground-truth CER vs the confidence obtained based on the CTC loss (left), and the confidence obtained using our augmentation based confidence metric (right). Our confidence metric assigns higher values to the lines with lower CER. Whereas, for the same CTC loss based confidence, high weights are assigned to the lines irrespective of their CERs, indicating a low correlation with correctness.}
%     \label{fig:iam_main_plot}
% \end{figure*}

% \begin{figure*}
%     \centering
%     \includegraphics[scale=0.25]{./plots_for_supp/cvl/main_plot.png}
%     \caption{\small \textbf{Correlation between correctness and confidence metric used on CVL} Plot of ground-truth CER vs the confidence obtained based on the CTC loss (left), and the confidence obtained using our augmentation based confidence metric (right). The CTC based metric assigns high confidence values to even those lines with high CER. Our CER based metric is more closely correlated with the error, as observed.}
%     \label{fig:cvl_main_plot}
% \end{figure*}

% \begin{figure*}
%     \centering
%     \includegraphics[scale=0.25]{./plots_for_supp/kohtd/main_plot.png}
%     \caption{\small \textbf{Correlation between correctness and confidence metric used on KOHTD} Plot of ground-truth CER vs the confidence obtained based on the CTC loss (left), and the confidence obtained using our augmentation based confidence metric (right). The CTC based metric assigns high confidence to lines irrespective of their CERs. The unnatural blockyness of the plot is because the evaluation on this dataset is at a word level, and hence there is an inherent quantization of possible CER. }
%     \label{fig:kohtd_main_plot}
% \end{figure*}


% % todo: kohtd remaining
% \section{Writer-specific Adaptation}
% Most of the datasets considered here, and in practice as well, generally consist of only lines from one writer, and thus one writing style. This helps the algorithm to learn from multiple cues across lines, and adapt to the writer's style. This becomes difficult when the same page has writing from multiple writers, as then the number of lines per writer decreases. To do this experiment, we concoct a dataset, where we create pages (i.e., list of lines) by randomly choosing lines from multiple pages (from different writers), without replacement. Then we run our TTA algorithm, except that now it sees lines from multiple writers at a time in a page. We present the performances in Figure \ref{fig:multiple_writers} for all the datasets. The x-axis and y-axis show the performance on the vanilla and concocted dataset. As we can see almost all the points lie above the equi-performance line, indicating that single writer specific adaptation works much better than having multiple writers in a single page. 
% %The multiple writer performance even degrades for corruptions where the performance are low, i.e., top-right of the plot.

% % \input{./tables_for_supp/multiple_writers}

% % \begin{figure}
% %     \centering
% %     \includegraphics[scale=0.45]{}
% %     \label{fig:icdar_mw}
% % \end{figure}

% % \begin{figure}
% %     \centering
% %     \includegraphics[scale=0.45]{}
% %     \label{fig:gnhk_mw}
% % \end{figure}

% % \begin{figure}
% %     \centering
% %     \includegraphics[scale=0.45]{}
% %     \label{fig:iam_mw}
% % \end{figure}

% \input{./tables_for_supp/icdar/topk}
% \input{./tables_for_supp/gnhk/topk}
% \input{./tables_for_supp/iam/topk}
% \input{./tables_for_supp/cvl/topk}
% \input{./tables_for_supp/kohtd/topk}

% \begin{figure*}
%     \centering
%     \includegraphics[scale=0.5]{./plots_for_supp/without_lm_comp.pdf}
%     \caption{\small \textbf{The role of LM in adapting the optical model for ICDAR2015-HTR and IAM respectively.} Each point here denotes the relative improvement the LM introduces for various corrupted versions of the dataset. The x value of each point is the CER improvement when decoding is done using the LM Decoder vs GreedyDecoder when evaluating the source model. The y-axis shows the CER improvement when our proposed method is used with the LM Decoder vs GreedyDecoder.}
%     \label{fig:lm_impact}
% \end{figure*}


% \begin{figure*}
%      \centering
%      \begin{subfigure}[b]{0.45\textwidth}
%          \centering
%          \includegraphics[width=\textwidth]{./images/icdar/mw.png}
%          \caption{ICDAR2015-HTR}
%          \label{fig:icdar_mw}
%      \end{subfigure}
%      \hfill
%      \begin{subfigure}[b]{0.45\textwidth}
%          \centering
%          \includegraphics[width=\textwidth]{./images/gnhk/mw.png}
%          \caption{GNHK}
%          \label{fig:gnhk_mw}
%      \end{subfigure}
%      \hfill
%      \begin{subfigure}[b]{0.45\textwidth}
%          \centering
%          \includegraphics[width=\textwidth]{./images/iam/mw.png}
%          \caption{IAM}
%          \label{fig:iam_mw}
%      \end{subfigure}
%      \hfill
%      \begin{subfigure}[b]{0.45\textwidth}
%          \centering
%          \includegraphics[width=\textwidth]{./images/cvl/mw.png}
%          \caption{CVL}
%          \label{fig:cvl_mw}
%      \end{subfigure}
%      \hfill
%      \begin{subfigure}[b]{0.45\textwidth}
%          \centering
%          \includegraphics[width=\textwidth]{./images/kohtd/mw.png}
%          \caption{KOHTD}
%          \label{fig:kohtd_mw}
%      \end{subfigure}
%     \caption{\textbf{Multiple writers in a single page.} Each point denotes results for each corrupted version of the particular dataset in the captions. The x-axis of each point is the performance on the vanilla dataset consisting of one writer per page, and the y-axis of that point shows the performance on the concocted version of the dataset consisting multiple writers in a page.}
%     \label{fig:multiple_writers}
% \end{figure*}




% % \input{./tables_for_supp/greedy_table} 



% % \begin{figure*}
% %     \centering
% %     \includegraphics[width=0.8\textwidth]{./images/icdar/short.png}
% %     \label{fig:icdar_short}
% % \end{figure*}
% % \begin{figure*}
% %     \centering
% %     \includegraphics[width=0.8\textwidth]{./images/icdar/long.png}
% %     \label{fig:icdar_long}
% % \end{figure*}

% % \begin{figure*}
% %     \centering
% %     \includegraphics[width=0.8\textwidth]{./images/gnhk/short.png}
% %     \label{fig:gnhk_short}
% % \end{figure*}
% % \begin{figure*}
% %     \centering
% %     \includegraphics[width=0.8\textwidth]{./images/gnhk/long.png}
% %     \label{fig:gnhk_long}
% % \end{figure*}

% % \begin{figure*}
% %     \centering
% %     \includegraphics[width=0.8\textwidth]{./images/iam/short.png}
% %     \label{fig:iam_short}
% % \end{figure*}
% % \begin{figure*}
% %     \centering
% %     \includegraphics[width=0.8\textwidth]{./images/iam/long.png}
% %     \label{fig:iam_long}
% % \end{figure*}
% % \begin{figure*}
% %     \centering
% %     \includegraphics[width=0.8\textwidth]{./images/iam/longer.png}
% %     \label{fig:iam_long}
% % \end{figure*}




% % {\small
% % \bibliographystyle{ieee_fullname}
% % \bibliography{egbib}
% % }





% \end{document}
