# Supplementary material for: Is it an i or an l: Test-time Adaptation of Text Line Recognition Models
Source: arXiv:2308.15037 source file (2023-08-29)
Supplement: Supplementary file 7 [file greedy_table.tex]

% Please add the following required packages to your document preamble:
% \usepackage[table,xcdraw]{xcolor}
% If you use beamer only pass "xcolor=table" option, i.e. \documentclass[xcolor=table]{beamer}
\begin{table*}[]
\centering
\resizebox{\textwidth}{!}{
\begin{tabular}{ccccccc}
\toprule
 &
  \multicolumn{6}{c}{Datasets} \\
  \midrule
\textbf{} &
  \multicolumn{2}{c}{ICDAR2015-HTR} &
  \multicolumn{2}{c}{GNHK} &
  \multicolumn{2}{c}{IAM} \\
  \midrule
\cellcolor[HTML]{FFFFFF}{\color[HTML]{202124} Corruptions} &
  \cellcolor[HTML]{FFFFFF} Source + Greedy &
  \cellcolor[HTML]{FFFFFF} TTA + Greedy &
   Source + Greedy &
  TTA + Greedy &
  Source + Greedy &
  TTA + Greedy \\
  \midrule
\cellcolor[HTML]{FFFFFF}{\color[HTML]{202124} original} &
  \cellcolor[HTML]{FFFFFF}16.2 &
  \cellcolor[HTML]{FFFFFF}15.2 &
  15.7 &
  \cellcolor[HTML]{FFFFFF}14.8 &
  to-do &
  7.0 \\
\cellcolor[HTML]{FFFFFF}{\color[HTML]{202124} brightness} &
  \cellcolor[HTML]{FFFFFF}16.1 &
  \cellcolor[HTML]{FFFFFF}15.0 &
  16.1 &
  \cellcolor[HTML]{FFFFFF}14.9 &
  to-do &
  8.2 \\
\cellcolor[HTML]{FFFFFF}{\color[HTML]{202124} contrast} &
  \cellcolor[HTML]{FFFFFF}17.5 &
  \cellcolor[HTML]{FFFFFF}17.0 &
  17.8 &
  \cellcolor[HTML]{FFFFFF}16.9 &
  to-do &
  7.9 \\
\cellcolor[HTML]{FFFFFF}{\color[HTML]{202124} defocus blur} &
  \cellcolor[HTML]{FFFFFF}42.8 &
  \cellcolor[HTML]{FFFFFF}85.3 &
  33.6 &
  \cellcolor[HTML]{FFFFFF}40.1 &
  to-do &
  27.9 \\
\cellcolor[HTML]{FFFFFF}{\color[HTML]{202124} elastic} &
  \cellcolor[HTML]{FFFFFF}44.6 &
  \cellcolor[HTML]{FFFFFF}79.7 &
  57.9 &
  \cellcolor[HTML]{FFFFFF}93.0 &
  to-do &
  94.7 \\
\cellcolor[HTML]{FFFFFF}{\color[HTML]{202124} fog} &
  \cellcolor[HTML]{FFFFFF}18.2 &
  \cellcolor[HTML]{FFFFFF}17.5 &
  19.2 &
  \cellcolor[HTML]{FFFFFF}18.0 &
  to-do &
  7.6 \\
\cellcolor[HTML]{FFFFFF}{\color[HTML]{202124} frost} &
  \cellcolor[HTML]{FFFFFF}32.5 &
  \cellcolor[HTML]{FFFFFF}55.5 &
  23.3 &
  \cellcolor[HTML]{FFFFFF}22.1 &
  to-do &
  13.3 \\
\cellcolor[HTML]{FFFFFF}{\color[HTML]{202124} gaussian blur} &
  \cellcolor[HTML]{FFFFFF}22.9 &
  \cellcolor[HTML]{FFFFFF}23.5 &
  24.9 &
  \cellcolor[HTML]{FFFFFF}26.4 &
  to-do &
  16.5 \\
\cellcolor[HTML]{FFFFFF}{\color[HTML]{202124} gaussian noise} &
  \cellcolor[HTML]{FFFFFF}29.3 &
  \cellcolor[HTML]{FFFFFF}30.1 &
  22.3 &
  \cellcolor[HTML]{FFFFFF}20.4 &
  to-do &
  8.4 \\
\cellcolor[HTML]{FFFFFF}{\color[HTML]{202124} glass blur} &
  \cellcolor[HTML]{FFFFFF}38.9 &
  \cellcolor[HTML]{FFFFFF}85.9 &
  40.9 &
  \cellcolor[HTML]{FFFFFF}37.9 &
  to-do &
  25.3 \\
\cellcolor[HTML]{FFFFFF}{\color[HTML]{202124} impulse noise} &
  \cellcolor[HTML]{FFFFFF}39.9 &
  \cellcolor[HTML]{FFFFFF}59.7 &
  25.0 &
  \cellcolor[HTML]{FFFFFF}23.3 &
  to-do &
  13.2 \\
\cellcolor[HTML]{FFFFFF}{\color[HTML]{202124} jpeg} &
  \cellcolor[HTML]{FFFFFF}30.3 &
  \cellcolor[HTML]{FFFFFF}28.6 &
  20.5 &
  \cellcolor[HTML]{FFFFFF}18.2 &
  to-do &
  8.2 \\
\cellcolor[HTML]{FFFFFF}{\color[HTML]{202124} motion blur} &
  \cellcolor[HTML]{FFFFFF}34.3 &
  \cellcolor[HTML]{FFFFFF}77.9 &
  37.0 &
  \cellcolor[HTML]{FFFFFF}35.1 &
  to-do &
  22.1 \\
\cellcolor[HTML]{FFFFFF}{\color[HTML]{202124} pixelate} &
  \cellcolor[HTML]{FFFFFF}29.6 &
  \cellcolor[HTML]{FFFFFF}26.6 &
  22.8 &
  \cellcolor[HTML]{FFFFFF}19.6 &
  to-do &
  11.5 \\
\cellcolor[HTML]{FFFFFF}{\color[HTML]{202124} saturate} &
  \cellcolor[HTML]{FFFFFF}16.2 &
  \cellcolor[HTML]{FFFFFF}15.2 &
  16.4 &
  \cellcolor[HTML]{FFFFFF}15.1 &
  to-do &
  6.9 \\
\cellcolor[HTML]{FFFFFF}{\color[HTML]{202124} shot noise} &
  \cellcolor[HTML]{FFFFFF}38.9 &
  \cellcolor[HTML]{FFFFFF}55.7 &
  25.2 &
  \cellcolor[HTML]{FFFFFF}23.7 &
  to-do &
  10.6 \\
\cellcolor[HTML]{FFFFFF}{\color[HTML]{202124} snow} &
  \cellcolor[HTML]{FFFFFF}26.2 &
  \cellcolor[HTML]{FFFFFF}26.5 &
  27.3 &
  \cellcolor[HTML]{FFFFFF}24.9 &
  to-do &
  15.7 \\
\cellcolor[HTML]{FFFFFF}{\color[HTML]{202124} spatter} &
  \cellcolor[HTML]{FFFFFF}17.9 &
  \cellcolor[HTML]{FFFFFF}17.2 &
  21.0 &
  \cellcolor[HTML]{FFFFFF}19.6 &
  to-do &
  7.7 \\
\cellcolor[HTML]{FFFFFF}{\color[HTML]{202124} speckle noise} &
  \cellcolor[HTML]{FFFFFF}41.0 &
  \cellcolor[HTML]{FFFFFF}59.9 &
  22.2 &
  \cellcolor[HTML]{FFFFFF}20.4 &
  to-do &
  10.4 \\
\cellcolor[HTML]{FFFFFF}{\color[HTML]{202124} zoom blur} &
   39.3 &
  \cellcolor[HTML]{FFFFFF} 95.5 &
   33.2 &
  \cellcolor[HTML]{FFFFFF}84.9 &
  to-do &
  96.2 \\
 \midrule
AVERAGE &
  \textbf{29.6} &
  \textbf{44.4} &
  \cellcolor[HTML]{FFFFFF}\textbf{26.1} &
  \cellcolor[HTML]{FFFFFF}\textbf{29.5} &
  \textbf{to-do} &
  \textbf{21.0} \\
  \bottomrule
\end{tabular}
}
\label{tabke:greedy}
\end{table*}
