# Supplementary material for: Is it an i or an l: Test-time Adaptation of Text Line Recognition Models
Source: arXiv:2308.15037 source file (2023-08-29)
Supplement: Supplementary file 13 [file multiple_writers.tex]

% Please add the following required packages to your document preamble:
% \usepackage[table,xcdraw]{xcolor}
% If you use beamer only pass "xcolor=table" option, i.e. \documentclass[xcolor=table]{beamer}
\begin{table}[]
\centering
\begin{tabular}{lccc} \\
\toprule
 & \multicolumn{3}{c}{Datasets}                                             \\
 \midrule
\multicolumn{1}{c}{} & \multicolumn{1}{c}{IC15-HTR} & \multicolumn{1}{c}{GNHK} & \multicolumn{1}{c}{IAM} \\
\midrule
{\color[HTML]{202124} original}        & 13.9 & 16.0          & 6.4           \\
{\color[HTML]{202124} brightness}      & 13.6 & 16.6          & 7.4           \\
{\color[HTML]{202124} contrast}        & 15.1 & 18.7          & 7.1           \\
{\color[HTML]{202124} defocus blur}   & 45.6 & 35.1          & 20.7          \\
{\color[HTML]{202124} elastic}         & 52.8 & 61.7          & 116.1         \\
{\color[HTML]{202124} fog}             & 15.8 & 19.1          & 7.2           \\
{\color[HTML]{202124} frost}           & 32.8 & 21.7          & 12.8          \\
{\color[HTML]{202124} gaussian blur}  & 20.9 & 25.0          & 13.7          \\
{\color[HTML]{202124} gaussian noise} & 23.1 & 20.2          & 7.5           \\
{\color[HTML]{202124} glass blur}     & 31.1 & 32.5          & 19.9          \\
{\color[HTML]{202124} impulse noise}  & 33.6 & 23.3          & 11.4          \\
{\color[HTML]{202124} jpeg}            & 22.7 & 17.8          & 7.7           \\
{\color[HTML]{202124} motion blur}    & 31.6 & 31.6          & 17.1          \\
{\color[HTML]{202124} pixelate}        & 20.4 & 20.2          & 9.0           \\
{\color[HTML]{202124} saturate}        & 14.1 & 18.8          & 6.3           \\
{\color[HTML]{202124} shot noise}     & 31.0 & 44.3          & 9.4           \\
{\color[HTML]{202124} snow}            & 23.2 & 24.7          & 13.7          \\
{\color[HTML]{202124} spatter}         & 14.7 & 19.1          & 7.0           \\
{\color[HTML]{202124} speckle noise}  & 32.1 & 20.5          & 9.1           \\
{\color[HTML]{202124} zoom blur}      & 44.4 & 65.6          & 36.5          \\
\midrule
Avg.                                               & 26.6                & 27.6 & 17.3 \\
\midrule
Single Writer (Avg.) & \textbf{23.9} & \textbf{22.5} & \textbf{13.6} \\
\bottomrule
\end{tabular}
\caption{Mixing lines from multiple writers for each of the datasets and their corrupted versions.}
\label{table:multiple_writers}
\end{table}
